# Supplementary material for: A Big Data Architecture Design for Smart Grids Based on Random Matrix Theory
Source: arXiv:1501.07329 source file (2015-06-16)
Supplement: Supplementary file 1 [file ArchAppendixarXiv.pdf]

# A Big Data Architecture Design for Smart Grids Based on Random Matrix Theory

Xing He, Qian Ai, *Member, IEEE,*, Robert C. Qiu, *Fellow, IEEE,*, Wentao Huang, Longjian Piao

***Abstract*—Data in smart grids with features of volume, velocity, variety, and veracity (i.e. 4Vs data) are difficult to handle by traditional tools, which are highly dependent on assumptions of specific roles or models with casual logics. This paper motivates big data analysis to process data from high-dimensional perspectives by using random matrix theory. An architecture combining smart grids and big data is proposed as a universal solution for control and operation in power systems. Based on this architecture, we are able to detect signals indicating sudden changes or faults in a power grid by comparing experimental findings with the random matrix theoretical predictions. Mean Spectral energy Radius (MSR) is defined as a new statistic to visualize the data correlations for this architecture. Comparative analysis of the MSRs from distributed regional centers under group-work mode is able to produce a contour line to locate the signal source even with data of imperceptible differences in low-dimensional perspectives. It demonstrates that some analyses are able to be extracted directly from the raw data which was hardly observable by conventional tools. Five case studies and their visualizations validate the effectiveness and higher performance of this designed architecture in various fields of smart grids. To our best knowledge, this study is the first attempt to design such a universal architecture for applying big data in smart grids.**

***Index Terms*—Big data, smart grid, architecture, random matrix, high dimension, 4Vs data, mean spectral energy radius**

## I. Introduction

BIG data is a new scientific trend [1, 2]. It reveals inherent correlations—once the correlations between causes and effects are established, statistical models, rather than physical ones, are built to gain insight to the mechanisms for control and prediction purposes. In other words, big data is more closely linked to a data processing technology with statistical correlations rather than physical models with casual logics or engineering solutions with specific simplifications and assumptions.

Big data is a new trend with lots of applications in mind. It has been successfully applied as a powerful analytic tool for numerous physical phenomena, such as quantum [3], financial systems [4, 5], biological systems [6], as well as wireless communication networks [7–9]. The connections between big data and these systems seem similar: two major tasks are 1) big data modeling, and 2) big data analysis. The 4Vs data (data with features of volume, variety, velocity, and veracity) [10] in smart grids, which were hard to handle within a tolerable elapsed time or hardware resources by traditional tools, has encouraged the development of an emerging and interesting field—Big Data researches for power system [11–13]. System architectures of big data applications in smart grids will appear as in other fields, for example, financial systems. After tying together smart grids and big data, we are able to crystallize many traditional problems and focus our efforts on their connection.

This work was supported by National Key Technology Research and Development Program of Science and Technology (2013BAA01B04).

Xing He, Qian Ai, Wentao Huang, Longjian Piao, Guanping Lu, Zhiwen Yu, Shiyi Wang are with the Department of Electrical Engineering, Shanghai Jiaotong University, Shanghai 200240, China (e-mail: hexing_hx@126.com; aiqian@sjtu.edu.cn)

Robert C. Qiu is with the Department of Electrical and Computer Engineering, Tennessee Technological University, Cookeville, TN 38505 USA (e-mail: rqiu@tntech.edu)

### A. Contribution

This paper demonstrates a new architecture to apply big data in smart grids as a statistical solution with universal processes. Firstly, we introduce the random matrix theory as our mathematic foundation. Then, a standard random matrix is formed in a systematical manner to map the measured or simulated data in power systems. Finally, we conduct matrices analysis and compare experimental findings with the theoretical predictions (i.e. the Marchenko-Pastur Law, the Kernel Density Estimation, and the Single-ring Law). Based on the above mathematical procedure, a new statistic—mean spectral energy radius (MSR)—is proposed to visualize the data correlations and clarify what should be interchanged among the grid components under the group-work mode. We also conduct five case studies based on this architecture and summarize the most interesting results. 1) The results of comparisons between experimental findings and the random matrix theory predictions are sensitive to events, as well as the proposed statistic MSR. In addition, there are some inherent relations for variety of data in high-dimensional perspectives. 2) There exists some relationships between the MSR and other engineering or mathematical parameters. 3) The data processing procedures of this architecture are used as a new method to find critical active power point at any bus node taking account of grid fluctuations. 4) Comparative analysis of the MSRs is able to generate a contour line to locate signal source even with data of imperceptible differences from distributed regional centers. 5) The architecture is suitable for not only the power flow analysis, but also the fault detection. To our best knowledge, our study represents the first such attempt in the literature on power systems.

### B. Related Work

It is well-established that data resource in power systems should be utilized much more efficiently. For example, Kanao et al. proposed a practical data utilization method based on

harmonic state-estimation (HSE) for power system harmonic analysis [14]. It was a data processing method in a specific field and only available when the engineering model is accurate. Alahakoon et al. proposed advanced analytic refer to a number of techniques which include a combination of data mining and knowledge discovery tools, machine learning technologies, and so on [15]. It required a lot of related sciences and technologies, however. Recently, Xu initiated power disturbance data analytics to explore useful aspects of power quality monitoring data and showed a wide applied scope in the future [16]. The mathematical foundations and system framework were missing yet. Although lots of researches were done about physical models in specific fields of power systems with according data utilization method, little attention has been paid to the architecture designed for power systems with solid mathematical foundations and universal statistical procedures. The rest of this paper is organized as follows. Section II describes the theoretical models based on random matrix theory. Section III proposes the big data architecture for power systems and demonstrates the advantages. Section IV presents five case studies based on the designed architecture in various fields of smart grids, after which some big data findings are compared with theoretical predictions proposed in Section II to detect signals from noises. Section V concludes the paper.

## II. From Random Matrix Theory to Big Data Analysis

### A. Random Matrix Theory

*1) Marchenko-Pastur Law (MP Law):*

The MP Law describes the asymptotic behavior of singular values of large rectangular random matrices. Let $\mathbf{X} = \{\xi_{ij}\}$ be a $N \times T$ ($N/T = c \in (0,1]$ ) random matrix whose entries are independent identically distributed (i.i.d.) variables with mean $\mu = 0$ and variance $\sigma^2 < \infty$. The empirical spectrum density (ESD) of the corresponding sample covariance matrix $\mathbf{S} = \frac{1}{T}\mathbf{X}\mathbf{X}^H$ (i.e. $f(\lambda_{\mathbf{S}})$) converges to the distribution of MP Law [17, 18] with density function:

$$f_{\text{MP}}(x) = \begin{cases} \frac{1}{2\pi x c\sigma^2}\sqrt{(b-x)(x-a)} & , a \leqslant x \leqslant b \\ 0 & , \text{otherwise} \end{cases} \quad (1)$$

where $a = \sigma^2(1-\sqrt{c})^2$, $b = \sigma^2(1+\sqrt{c})^2$, $c = N/T$.

*2) Kernel Density Estimation (KDE):*

A nonparametric estimate [19] of the empirical spectral density of the sample covariance matrix is used

$$f_n(x) = \frac{1}{nh}\sum_{i=1}^{n} K(\frac{x-\lambda_i}{h}) \quad (2)$$

where $\lambda_i$ $(i = 1, 2, \cdots, n)$ are the eigenvalues of $\mathbf{S}$, and $K(\cdot)$ is the kernel function for bandwidth parameter $h$.

*3) The Single-Ring Law:*

For each $n \geqslant 1$, let $\mathbf{A}_n$ be a random matrix which admits the decomposition:

$$\mathbf{A}_n = \mathbf{U}_n \mathbf{T}_n \mathbf{V}_n \quad , \mathbf{T}_n = \text{diag}(s_1, \cdots, s_n) \quad (3)$$

where ${s_i}^H s_i$ are positive, and $\mathbf{U}_n$ and $\mathbf{V}_n$ are two independent random unitary matrices which are Haar-distributed independently from $\mathbf{T}_n$. In probability, the ESD of $\mathbf{A}_n$ converges weakly to a deterministic measure whose support is under certain mild conditions [20]. Some outliers to single ring law [21] are observed.

Consider the matrices product $\tilde{\mathbf{Z}} = \prod_{i=1}^{L} \mathbf{X}_{u,i}$, where $\mathbf{X}_u$ is the singular value equivalent [22] of the rectangular $N \times T$ non-Hermitian random matrix $\tilde{\mathbf{X}}$, whose entries are independent identically distributed (i.i.d.) variables with mean $\mu(\tilde{\mathbf{x}}_{k,:}) = 0$ and variance $\sigma^2(\tilde{\mathbf{x}}_{k,:}) = 1$ for $k = (1, 2, \cdots, N)$. The matrices product $\tilde{\mathbf{Z}}$ is converted to $\mathbf{Z}$ by a transform which make the variance to $\sigma^2(\mathbf{z}_{:,k}) = 1/N$ for $k = (1, 2, \cdots, N)$. Thus, the empirical spectrum density of $\mathbf{Z}$ converges almost surely to the same limit given by

$$f_{\mathbf{Z}}(\lambda) = \begin{cases} \frac{1}{\pi c \alpha}|\lambda|^{(2/\alpha - 2)} & , (1-c)^{\alpha/2} \leqslant |\lambda| \leqslant 1 \\ 0 & , \text{otherwise} \end{cases} \quad (4)$$

as $N, T \to \infty$ with the ratio $N, T = c \in (0, 1]$. On the complex plane of the eigenvalues, the inner circle radius $r_{\min\_\lambda(\mathbf{z})}$ is $(1-c)^{\alpha/2}$ and outer circle radius is unity. Moreover, $\mathbf{S} = \mathbf{Z}\mathbf{Z}^H$ is able to acquired and its ESD converges to the the distribution of MP Law.

### B. Big Data Analysis

Currently, there exists no general standardized definition for Big Data. In this paper, we give a mathematical definition below used in the past work [7–9, 17]

- Data samples are modeled as vectors, say $\mathbf{x}_1, \mathbf{x}_2, \cdots, \mathbf{x}_n$;
- The number of data samples, say $n$, is large;
- A function $f(\mathbf{x}_1, \mathbf{x}_2, \cdots, \mathbf{x}_n)$ is defined using $n$ random vectors;

In the power systems, lots of raw data $\hat{x}$ are acquired by observations or simulations; for a certain time $t_i$, they are arranged as a vector $\hat{\mathbf{x}}_{t_i}$. As time goes by, vectors are acquired one by one and a sheet is naturally formed as data set to map the systems. Any arbitrary section in the set is available as raw data source $\mathbf{\Omega}\hat{\mathbf{x}}$ for further analyses. Thus, the $\mathbf{\Omega}\hat{\mathbf{x}}$ consists of sample vectors on a series of times denoted as $\hat{\mathbf{x}}_{t_1}, \hat{\mathbf{x}}_{t_2}, \cdots, \hat{\mathbf{x}}_{t_i}, \cdots$; at any time $t_i$, the vector $\hat{\mathbf{x}}_{t_i}$ comprises sample data denoted as $x_{t_i,n_1}, x_{t_i,n_2}, \cdots, x_{t_i,n_i}, \cdots$ . The length of $n$ is decided by the number of variables at a single sampling time, and the length of $t$ is subject to the volume of historical data set and is generally big enough.

For the raw data source $\mathbf{\Omega}\hat{\mathbf{x}}$, we can focus on any data area as a split-window to form a raw matrix $\hat{\mathbf{X}}$. Then, it is converted to a standard non-Hermitian random matrix $\tilde{\mathbf{X}}$ by a normalization which is performed line-by-line with following algorithms:

$$\tilde{x}_{ij} = (\hat{x}_{ij} - \overline{\hat{\mathbf{x}}_i}) \times (\sigma(\tilde{\mathbf{x}}_i)/\sigma(\hat{\mathbf{x}}_i)) + \overline{\tilde{\mathbf{x}}_i}, 1 \leqslant i \leqslant N; 1 \leqslant j \leqslant T \quad (5)$$

where $\hat{\mathbf{x}}_i = (\hat{x}_{i1}, \hat{x}_{i2}, \cdots, \hat{x}_{iT})$ and $\overline{\tilde{\mathbf{x}}_i} = 0$, $\sigma^2(\tilde{\mathbf{x}}_i) = 1$.

The matrix $\mathbf{X}_u \in \mathbb{C}^{|N \times N}$ is introduced as the singular value equivalent of the matrix $\tilde{\mathbf{X}} \in \mathbb{C}^{|N \times T}$ by

$$\mathbf{X}_u = \mathbf{U}\sqrt{\tilde{\mathbf{X}}\tilde{\mathbf{X}}^H} \quad (6)$$

where $\mathbf{U} \in \mathbb{C}^{|N \times N}$ and ${\mathbf{X}_u}^H \mathbf{X}_u \equiv \tilde{\mathbf{X}}\tilde{\mathbf{X}}^H$.

Then, the matrices product $\tilde{\mathbf{Z}} = \prod_{i=1}^{L} \mathbf{X}_{u,i}$ is acquired, based on which $\mathbf{Z}$ is calculated row-by-row with following formula:

$$\mathbf{z}_j = \tilde{\mathbf{z}}_j / (\sqrt{N}\sigma(\tilde{\mathbf{z}}_j)) \quad , 1 \leqslant j \leqslant N \tag{7}$$

where $\mathbf{z}_j = (z_{1j}, z_{2j}, \cdots, z_{Nj})^T$ , $\tilde{\mathbf{z}}_j = (\tilde{z}_{1j}, \tilde{z}_{2j}, \cdots, \tilde{z}_{Nj})^T$.

With the variable transformation above, the matrix $\mathbf{Z}$ is acquired. Furthermore, we calculate the mean value of the radius for all the eigenvalues of $\mathbf{Z}$ on the complex plane as a new high-dimensional statistic $\kappa_{\text{MSR}}$ (i.e. $\kappa_{\text{MSR}} = \overline{r_{\lambda(\mathbf{Z})}}$).

In general, we conduct high-dimensional analysis to reveal the statistical properties of the raw data $\hat{x}$. $\mathbf{Z}$ and its empirical spectrum density are analyzed based on the newly developed Single-ring Law, and the high-dimensional statistic $\kappa_{\text{MSR}}$ is calculated and visualized. In addition, the corresponding sample covariance matrix $\mathbf{S} = \frac{1}{T}\mathbf{Z}\mathbf{Z}^H$ is calculated for further analyses by using the histogram, the KDE, and the MP Law.

## III. A Big Data Architecture for Smart Grids and its Advantages

### A. Big Data Architecture for Smart Grids

The architecture consists of two independent procedures to connect smart grids and big data: big data modeling as an engineering procedure for the smart grids, and big data analysis as a mathematical procedure for the big data, respectively. The frequently used notations are shown in Table I.

TABLE I: Some Frequently Used Notations

| *Notations* | *Means* |
|---|---|
| $\mathbf{A}_{\text{Time}}$ | time area to focus on the data split-window |
| $T_{\text{Len}}$ | length of $\mathbf{A}_{\text{Time}}$ |
| $\zeta$ | sample points number in a window, equals to $T_{\text{Len}}$ |
| $\mathbf{A}_{\text{Node}}$ | node area to focus on the data split-window |
| $N_{\text{Len}}$ | length of $\mathbf{A}_{\text{Node}}$ |
| $t$ | time: $t_0$ for current time, $t_s$ for sampling time |
| $\mathbf{X}$ | matrix in the split-window: $\hat{\mathbf{X}}$ for raw data, $\tilde{\mathbf{X}}$ for transition, $\mathbf{X}$ for singular value equivalent |
| $\mathbf{S}$ | corresponding sample covariance matrix of $\mathbf{X}$ |
| $P_{\text{Bus-}n}$ | power demand of load at bus-n |
| $P_{\text{max\_Bus-}n}$ | critical point on $P_{ower}$-$V_{oltage}$ curve for bus-n |
| $\gamma_{\text{Acc}}$ | addition factor for load fluctuation of the grid |
| $\gamma_{\text{Mul}}$ | multiplication factor for load fluctuation of the grid |

The designed architecture for smart grids is illustrated in Fig. 1. The raw data source $\mathbf{\Omega}\hat{\mathbf{x}}$ is acquired during the engineering procedure as described in Section II. Then we conduct following steps as the mathematical procedure to extract analyses:

Especially, in step *2) Focus on the data window*, if the last edge of the sampling time area is current time (i.e. $\mathbf{A}_{\text{Time}}(\text{end}) = t_0$), we focus on a real-time data window. Besides, as the split-window in fixed size slides across data source area with $t_\Omega$ set in *1b)*, a series of $\kappa_{\text{MSR}}$ will be got for further research and visualization.

### B. Advantages in Algorithm for Data Processing

This architecture analyzes data from high-dimensional perspectives. The solid purple lines in Fig. 3 illustrates the four

**Steps of Mathematical Procedure**

1) Set the initial parameters
   1a) Set $\mathbf{A}_{\text{Time0}}$ and $\mathbf{A}_{\text{Node0}}$ to focus on the first data window
   1b) Set $t_\Omega$ and $k=0$ to slide the moving split-window (MSW)
2) Focus on correspond window to form $\hat{\mathbf{X}}$ ($\mathbf{A}_{\text{Time}} = \mathbf{A}_{\text{Time0}} + k$)
3) Convert the raw matrix $\hat{\mathbf{X}}$ to standard random matrix $\tilde{\mathbf{X}}$
4) Calculate $\mathbf{X}_u$, $\tilde{\mathbf{Z}}$, $\mathbf{Z}$, $\mathbf{S}$
5) Calculate the eigenvalues and do empirical spectrum density analysis
6) Calculate the $\kappa_{\text{MSR}}$
7) Visualize results
8) Judge as times goes by:
   8a) $k < t_\Omega \Rightarrow k{+}{+}$; back to *step 2)*
   8b) $k \geqslant t_\Omega \Rightarrow$ END)

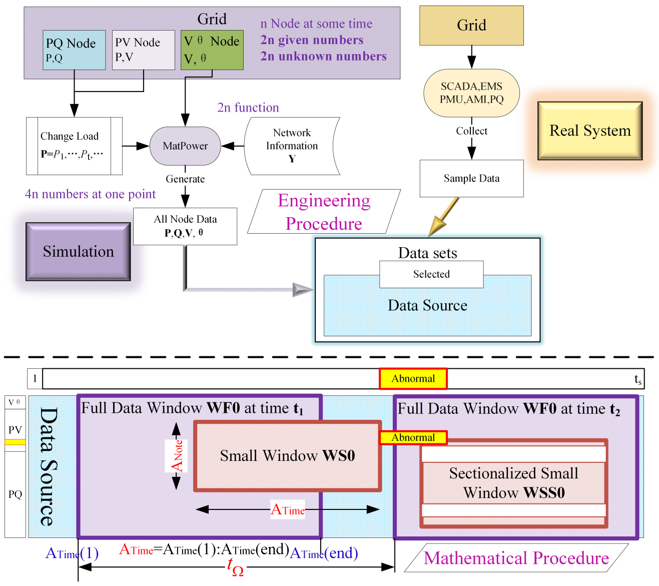


Fig. 1: The designed big data architecture for smart grids. The part above the dot line illustrates an engineering procedure for big data modeling, during which the raw data source $\mathbf{\Omega}\hat{x}$ are formed to map the physical system. The other part below the dot line illustrates a mathematical procedure for big data analysis. It is fully independent of engineering parameters, and during which the analyses are extracted directly from the raw 4Vs data $\hat{x}$.

**Steps of Data Management for G3**

1) Form standard random matrices $\tilde{\mathbf{X}}$
2) Acquire $\mathbf{Z}$, $\mathbf{S}$ by variables transforming ($\tilde{\mathbf{X}} \to \mathbf{X}_u \to \tilde{\mathbf{Z}} \to \mathbf{Z} \to \mathbf{S}$)
3) Calculate eigenvalues of $\mathbf{Z}$ and do ESD analysis for $\mathbf{S}$, and Calculate $\kappa_{\text{MSR}}$ with time goes by. Visualize and compare the results with the random matrix theory to conduct high-dimensional analysis
4) Conduct engineering interpretations

steps of the data management in this architecture. It is a universal procedure as follows:

On the other hand, the procedure of traditional data processing algorithms relies highly on specific simplifications and assumptions to build models. Taking genetic algorithm for an example, two steps are required to achieve the result. The first step is to transcode the engineering variables to gene as input for the gene model, which is based on hypothesis for the specific roles of the engineering systems. The second step is to perform the genetic algorithm through selection, crossover and mutation operations. During these operations, however, the problems such as improper settings of the size

of the population, or the probabilities of the crossover or the mutation, will inevitably make the result worse.

Compared to traditional algorithms, big data analysis enable us to analyze the interrelation and interaction seen as correlations directly from the raw data. It is a pure mathematic procedure without subjective assumptions, physical models, or causal logics. As a result, they are easier in logic and faster in speed. Moreover, except step *4): Conduct Engineering Interpretation*, the whole procedure are objective without introducing or accumulating the system errors; besides, the accidental errors can be eliminated either with the random matrix size growing, or by repletion test and parallel computing as a result of the independence of the algorithm.

### *C. Advantages in Managing Mode for Grid Operation*

Generally, the power grids evolutions are summarized as three generations—G1, G2, and G3 [23]. Their own network structures are depicted in Fig. 11 [24]. In addition, their data flows and energy flows, as well as corresponding data management systems and work modes, are quite different [25], as detailed in Fig. 2 and Fig. 3, respectively. We will discuss the background and basic information, as well as the managing mode for G1, G2, and G3 in details. It will come to a conclusion that the group-work mode based on the big data architecture is the trend for smart grids.

G1 was developed from around 1900 to 1950, featured by small grids. For G1, components interchange energy and data within the isolated grid to keep system stability. The components are fully controlled by decentralized control system and operating under individual-work mode. It means that each apparatus collects designated data and makes corresponding decisions only with its own application, just as shown at the above part of Fig. 11a. The G1 individual-work mode works with an easy logic and little information communication. Whereas, it means few advanced functions and inefficient utilization for data resources. It is only suitable for small isolated grids.

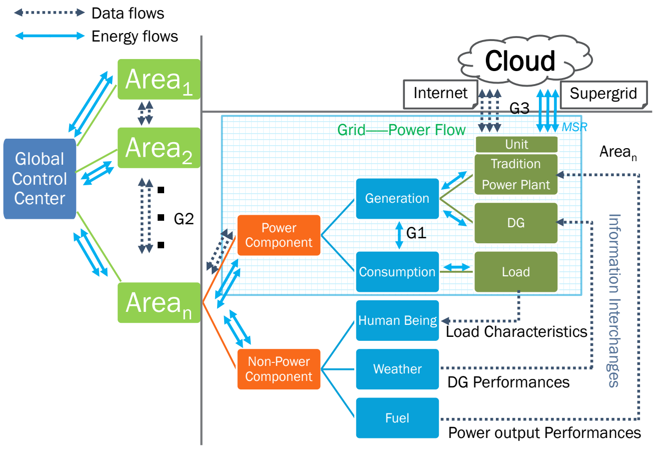


Fig. 2: Data flows and energy flows for three generations of power systems. The single lines, double lines, and triple lines indicate the flows of G1, G2, and G3, respectively.

G2 was developed from about 1960 to 2000, featured by large-scale interconnected grids. For G2, components interchange data and energy within the adjacent grids. The components are dispatched by control center and operating under team-work mode. The regional team leaders, likes local dispatching centers, substations, or microgrid control centers, aggregate their own team-members (i.e. components in the region) into a standard black-box model. These standard models will be further aggregated by the global control center for the overall rather than the specific control or prediction purposes. The two aggregations above are achieved by four steps, which are data monitoring, data pre-processing, data storage, and data processing, respectively. However, lots of engineering technologies or sciences have to be investigated as the foundations of the G2 team-work mode—Cognitive Radio Wireless Network [26–28], Specific Communication Service Mapping (SCSM) as Information and Communication Technology (ICT) [29], Cloud Storage, Parallel Computing as Computer Science (CS), and Modelling Building, Parameter Identification as Mathematical Modeling [30, 31]. The description above are illustrated by dotted blue lines in Fig. 3. In general, the G2 team-work mode aims to make accurate engineering models with specific parameters based on many technologies and sciences. Therefore, it will not work well for G3 with 4Vs data as described in Section I.

The development of G3 was launched at the beginning of the 21st century, and expected to be completed over 2050. Fig. 11c shows that the clear-cut partitioning is no longer suitable for G3, as well as the G2 team-work mode which is based on the regional leader. For G3, the control force of the regional center (if still exist) is greatly released by individual units. The high performance and self-control individuals results in much more flexible flows to improve utilization by sharing resources among the whole grid. Accordingly, the group-work mode is proposed. Under this mode, the individuals play a dominant part under the authority of the global control centers [25]; and VPPs (Virtual Power Plants) [32], MMGs (multi-microgrids) [33], for instance, typically operate under this mode. It provides a relaxed environment to benefit both the individuals and the grids: the formers, driven by their own interests and characteristics, create or join a relatively free group to benefit mutually from sharing advantageous resources; meanwhile, the groups, such as VPPs and MMGs, are generally big and controllable enough to be good customer or managers to assist the latters (i.e. the smart grids).

## IV. FIVE CASE STUDIES

For the following designed experiments, all the data are obtained in two scenarios: 1) Only noises (i.e. benchmark, whose statistical results agree with the MP Law and the Ring Law); 2) Signals plus noises. In the following five cases, we treat small random loads fluctuations and sample errors as white noises, and sudden changes or faults as signals.

Case 1 to Case 4, based on Matpower, belongs to the field of power system stability and control; Case 5, based on PSCAD/EMTDC, is about fault detection. Case 1 is a simple study to validate that big data is able to quickly detect the signals from the noises with the real time data

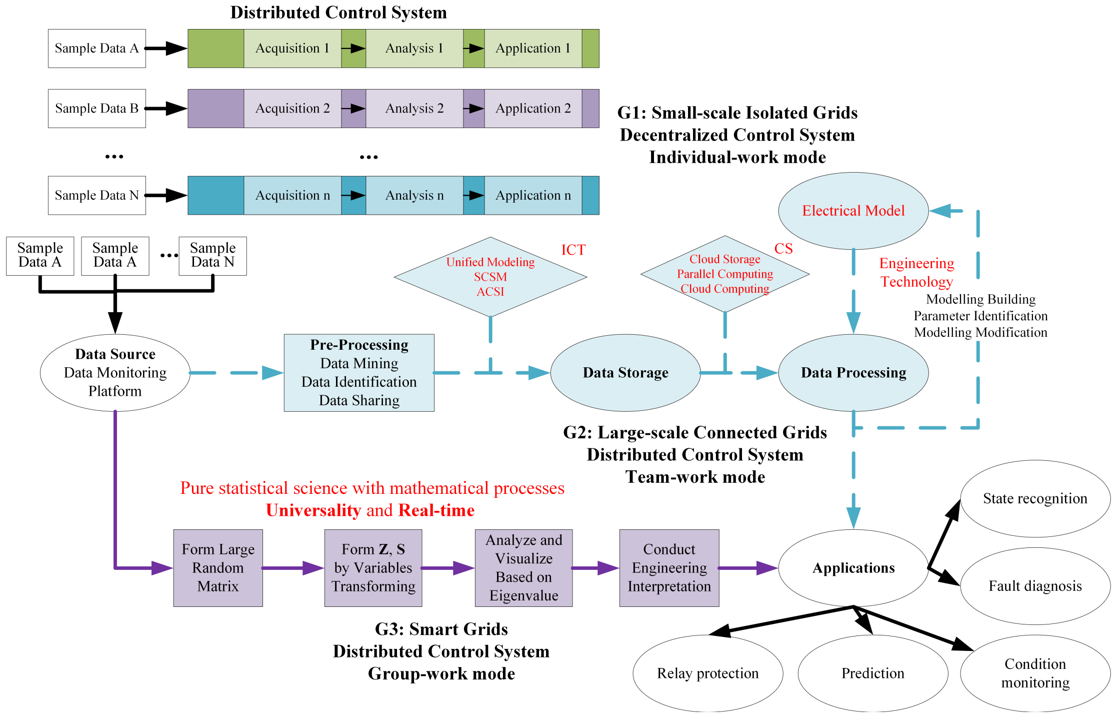


Fig. 3: Data management systems and work modes for three generations of power systems. The above, middle, and below parts indicate the data management systems and the work modes of G1, G2, and G3, respectively. For G1, each grid works independently. For G2, global and local control centers are operating under the team-work mode. For G3, the group-work mode breakthrough the regional limitation for energy and data flows and have a better performance.

flow. Case 2 studies the relationships between the statistic MSR and other engineering or mathematic parameters. Case 3 proposes a new method based on case 2 to calculate critical active power point. Case 4 is an advanced application for the proposed big data architecture: extracting useful analyses which are hardly observed in low-dimensional perspectives by comparative analysis of MSRs from different regional centers under group-work mode. Case 5 shows that the architecture is also suitable for other fields in power systems such as fault detection.

### *A. Case 1: Observation from the Split-Window with Full Network and 500 Sample Points—$N_{Len}=118$, $\zeta=500$*

The grid is a standard IEEE 118-bus system with six partitions displayed as Fig. 12 [34]. Detailed information about the test bed is referred to the *case118.m* in *Matpower package* and *Matpower 4.1 Users Manual* [35]. Case 1 is a simple case to validate the effectiveness of the designed architecture.

Let $N=118$, $t=500$, $c=N/T=0.236$, as typical value. Thus each split-window has $n=NT=59,000$ data. Table II shows the series of assumed events, and the accordingly data visualization and MSR are depicted as Fig. 4 and 5, respectively.

*1) Sampling time $t_s=550$ s, Time Area $\mathbf{A}_{Time}=51:550$ s:*

There are only small load fluctuations in this split-window, which means that white-noises play a dominant part. Then, we compare the histogram, the KDE and the MP Law. Inspection of Fig. 4a indicates that, in a white-noises dominated system, the kernel density estimation (in red line) matches the histogram (in blue bar) very well. Moreover, the histogram curve and the KDE curve agree with MP Law (in blue line).

*2) Sampling time $t_s=551$ s, Time Area $\mathbf{A}_{Time}=52:551$ s:*

For this split-window, Fig. 4b shows that the eigenvalues of the Ring-Law collapse to the circle center, and both the histogram and the KDE deviate from the MP Laws. According to the MP Laws, there are some signals in the system—any deviation of the benchmark (white noises only) indicates the presence of signal. Indeed, just at time $t=551$ s, the $P_{\text{Bus-59}}$ suddenly changes from 0 MW to 200 MW somehow.

Fig. 5 depicts that the $\kappa_{\text{MSR}}$ change dramatically in a short time. As the length of time area $\zeta=500$, time $t=551$ s when the step change is occurring as the signal is included during all the sampling times from $t_s=551$ s to $t_s=1049$ s. It results in the deviation $(0.9368, 0.8081, 0.7757, \cdots)$. At the sampling time $t_s=1050$ s when the time area $\mathbf{A}_{\text{Time}}=551:1050$ s, however, the step signal is no longer exist, as well as the deviation of the histogram and the KDE from the MP Law, and the $\kappa_{\text{MSR}}$ is back to 0.9320.

In addition, it is found that $\kappa_{\text{MSR}}$ for the data of $V$ (red line) which has definite physical meaning, and of $V+i\theta$ (black line) without any physical meaning, have the same trend. It indicates that MSR is a high-dimensional statistic which is independent of physical model and causal logic in some way. The green line indicates the inner radius of the single ring for the analyzing matrix, whose value is fully depended on the matrix size as formula 4 in section II.

This case indicates that the presented statistic MSR is sensitive to events, and there are some inherent relations for the variety of data. In general, it illustrates that real-time

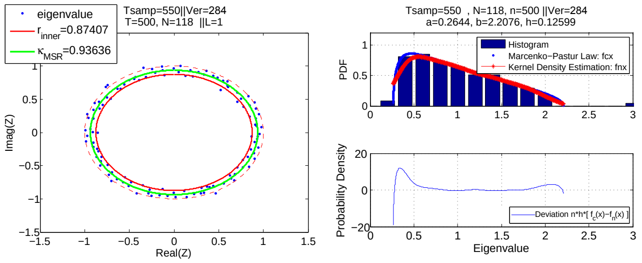


(a) $t_s = 550$ s

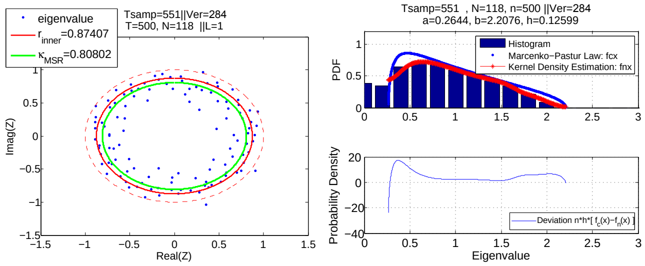


(b) $t_s = 551$ s

Fig. 4: Ring Law, and the Comparation among Histogram, KDE, and MP Law at Different Sampling times for Case 1

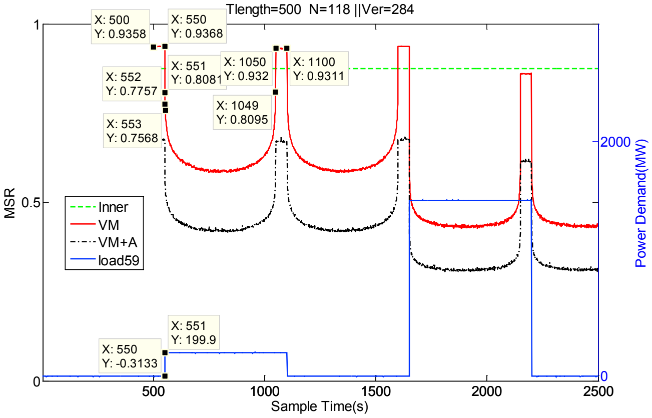


Fig. 5: MSR at Different Sampling times for Case 1

analysis can be carried out with less kinds of data under high-dimensional perspectives.

## *B. Case 2: Observation from the Smaller Split-Window with Full Net-work and 240 Sample Points—$N_{Len} = 118$, $\zeta = 240$*

Case 2 is similar to the previous one except that $\zeta$ is changed to 240 s, and the events are rearranged. In this case, we try to find the relationships between the MSR and the engineering parameters. The series of assumed events and $\kappa_{\rm MSR}$-$t$ curve are depicted as Table III and Figure 6, respectively.

a) During one step-change, there is a negative correlation between the min value of the MSR (i.e. $\kappa_{\rm MSR}$) and the step-change value of $P_{\rm Bus\text{-}59}$ (i.e. $\Delta P_{\rm Bus\text{-}59}$):

| | | | | | |
|---|---|---|---|---|---|
| $\Delta P_{\rm Bus\text{-}59}$ | 200 | 50 | 550 | 1650 | $\cdots$ |
| $P_{\rm Bus\text{-}59}$ | $0 \to 200$ | $200 \to 250$ | $250 \to 800$ | $850 \to 2500$ | $\cdots$ |
| $\kappa_{\rm min\_MSR}$ | 0.5562 | 0.6522 | 0.4689 | 0.3695 | $\cdots$ |

b) When the $P_{\rm Bus\text{-}59}$ is steady at a higher level, the $\kappa_{\rm MSR}$ is steady at a lower level:

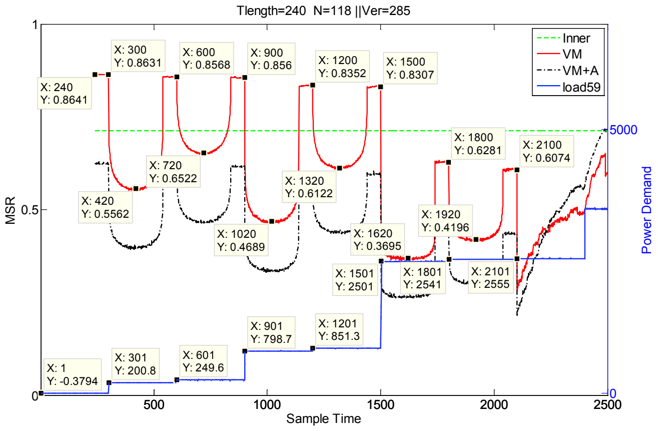


Fig. 6: MSR at Different Sampling times for Case 2

| | | | | | | |
|---|---|---|---|---|---|---|
| $P_{\rm Bus\text{-}59}$ | 0 | 200 | 250 | 800 | $\cdots$ | 2540 |
| $\kappa_{\rm MSR}$ | 0.8631 | 0.8568 | 0.8560 | 0.8352 | $\cdots$ | 0.6074 |

c) When the $P_{\rm Bus\text{-}59}$ approaches to the critical active power point $P_{\rm max\_Bus\text{-}59}$, a litter step change of the $P_{\rm Bus\text{-}59}$ will lead to a small value of the $\kappa_{\rm min\_MSR}$. The feature b) and c) is available to conduct vulnerable node identification [36] as a new method.

| | | | |
|---|---|---|---|
| $\Delta P_{\rm Bus\text{-}59}$ | 50 | 50 | 40 |
| $P_{\rm Bus\text{-}59}$ | $200 \to 250$ | $800 \to 850$ | $2500 \to 2540$ |
| $\kappa_{\rm min\_MSR}$ | 0.6522 | 0.6122 | 0.4196 |

d) When the $P_{\rm Bus\text{-}59}$ is beyond the $P_{\rm max\_Bus\text{-}59}$ (i.e. $P_{\rm Bus\text{-}59} > 2555$ MW), the $\kappa_{\rm MSR}$ is no longer steady.

## *C. Case 3: Critical Power Point Estimation*

This case designed as a new method to find the critical point $P_{{\rm max\_Bus\text{-}}n}$ based on the feature c) and d) of the previous one. In addition, grid fluctuations are set by $\gamma_{\rm Acc}$ and $\gamma_{\rm Mul}$

$$\tilde{y}_{{\rm load\_}nt} = y_{{\rm load\_}nt} \times (1 + \gamma_{\rm Mul} \times x_1) + \gamma_{\rm Acc} \times x_2 \qquad (8)$$

where $x_1$ and $x_2$ are random numbers from a standard Gaussian Distribution. By this model, the critical point $P_{{\rm max\_Bus\text{-}}n}$ at any designated node is able to be estimated even taking account of the grid fluctuations. In this model, the increase of grid fluctuations means the decrease of signal-noise ratio, which will cause a raise of the $\kappa_{\rm min\_MSR}$. Meanwhile, it will also cause the decrease of the $P_{{\rm max\_Bus\text{-}}n}$ for a certain node (2555 MW, 2548 MW, 2521 MW) which is commonsensible, just as show in Fig. 7.

## *D. Case 4: Group-work Mode*

For the above three cases, similar results can be achieved by analyzing raw data in low-dimensional perspectives. These cases validate the effectiveness of the designed architecture. In Case 4, however, we will design a case which can hardly be solved by traditional tools. It is based on the power system with 6 partitions (A1 to A6) depicted in Fig. 12. A PQ node far from slack bus is chosen as signal source, for example, bus-117 in area A1. It is much more vulnerable than PV nodes such as

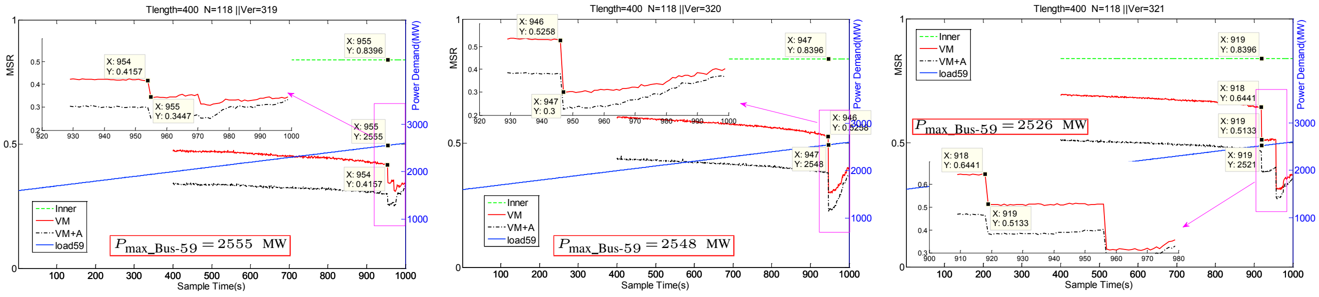


(a) $\gamma_{\text{Acc}} = 0,\ \gamma_{\text{Mul}} = 0$ (b) $\gamma_{\text{Acc}} = 1,\ \gamma_{\text{Mul}} = 0.02$ (c) $\gamma_{\text{Acc}} = 5,\ \gamma_{\text{Mul}} = 0.1$

Fig. 7: Critical Power Point Estimation Taking Account of Grid Fluctuations

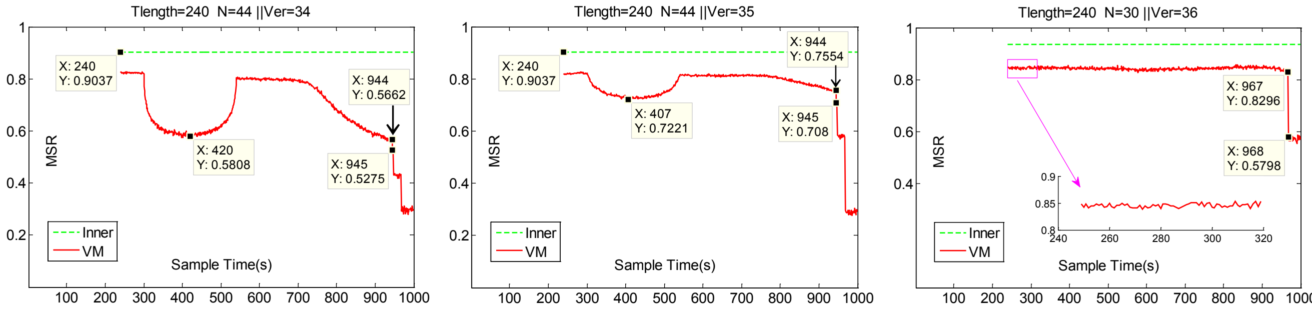


(a) $\mathbf{A}_{\text{Node}}$=[A1,A2] (b) $\mathbf{A}_{\text{Node}}$=[A3,A5] (c) $\mathbf{A}_{\text{Node}}$=[A4,A6]

Fig. 9: MSR of Union Regions

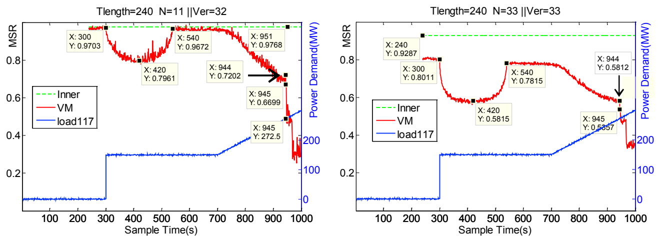


(a) $\mathbf{A}_{\text{Node}}$=A1 (b) $\mathbf{A}_{\text{Node}}$=A2

Fig. 8: MSR of Single Partitioning

bus-59. This case study is based on the proposed group-work mode. With the same procedures of the former case studies, the events set as signals, the load fluctuations set of the grid as white noises, and the $P_{\text{max\_Bus-117}}$ and the $\kappa_{\text{MSR}}$-$t$ curve for the whole gird network are depicted by Table IV, Fig. 13, and Fig. 14, respectively.

Just like the global center, each local one calculates the MSR with data from its own region, such as Fig. 8a for A1, and 8b for A2. When the dada split-window is not big, just as A1 which only has 11 nodes (i.e. $N = 11$), although the signal is detected, the curve is not smooth. Thus, some areas are combined to smooth the $\kappa_{\text{MSR}}$-$t$ curve as Fig. 9a for A1&A2, 9b for A3&A5, and 9c for A4&A6, respectively. At last, Fig. 15a, 15b gives the raw data of $\hat{\mathbf{V}}$ and their low-dimensional visualization for all PQ buses in A3&A5 around sampling time $t_s = 301$ s when the small step-change of $P_{\text{Bus-117}}$ happened as signal.

Fig. 14 shows that the critical point is $P_{\text{max\_Bus-117}} = 272.5$ MW at $t_s = 945$ s. This point is observed by all the regional centers as shown in Fig. 8 and 9. Also, a signal occurring just at time $t = 301$ s is detected in the system. According to the $\kappa_{\text{MSR}}$ of Fig. 9a, 9b and 9c, it is found that to response to the signal at $t = 301$ s, the distribution of $\Delta\kappa_{\text{MSR}}$ in distributed regions is just like the contour line and the A1&A2 is the mountaintop. As a result, we conjecture that the system signal is generated at A1&A2 rather than A3&A5 or A4&A6. The events set in Table IV validates the conjecture.

Under the group-work mode, by the interchanges of the regional high-dimensional statistic MSRs, some useful analyses are extracted directly from the raw data $\hat{V}$. Especially, for the raw voltage amplitude data set $\mathbf{\Omega}\hat{V}$ of A3&A5 as shown detailed in Fig. 15, the low-dimensional statistics—either one-dimensional Mean or two-dimensional Variance—changes too little to be utilized by using traditional data analysis tools.

### *E. Case 5: Fault Detection for Active Distribution Network*

This case shows the application of the designed architecture in another field of power systems. Faults and disturbances detection has become increasingly complicated in active distribution networks, due to the integration and variation of renewable generators and energy storage units [37]. Table V sets the events series and Fig. 16 illustrates the fault mode as the background of this case.

Fig. 10 indicates that some signals are detected by the $\kappa_{\text{MSR}}$-$t$ curve. Especially, it is conjectured that the most influent events are happening around $t = 3,000$ ms and $t = 13,000$ ms,

which means that the three-phase and line-to-line short circuit has more influence than the single-phase one. Due to space limitations, the fault identification and analyses extraction from the raw data sets $\mathbf{\Omega}\hat{V}$ are not discussed detailed. This case just shows that the architecture is also compatible with the protection field in power systems.

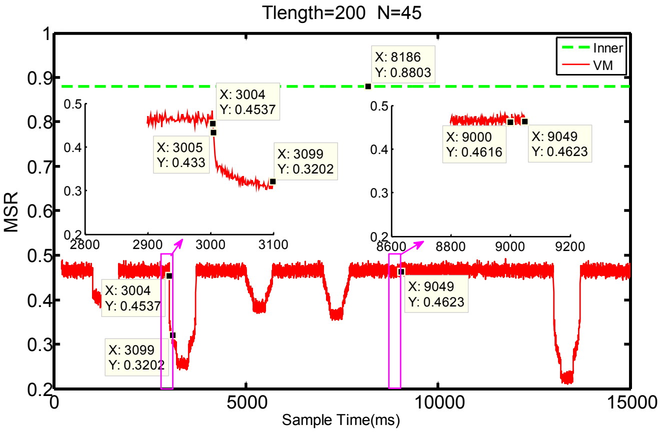

Fig. 10: MSR on Time Series for Failure Events

## V. Conclusion

This paper proposed a new big data architecture based on random matrix theory to connect smart grids and big data. This architecture consists of two independent procedures, which are big data modeling with an engineering procedure for the smart grids, and big data analysis with a mathematical procedure for the big data, respectively. In addition, moving split-window technology was used for real-time analysis, and a new statistic mean spectral energy radius was proposed to clarify what should be interchanged among the units under group-work mode. The algorithm of this architecture is based on a fixed objective procedure which is easier in logic and faster in speed. The architecture is universal, independent and flexible in managing smart grids. In addition, five case studies and their visualizations were designed to validate the performance of the designed architecture in various fields of smart grids.

However, some questions are still left. For example, to figure out the relationships between the mean spectral energy radius MSR and the physical parameters is a long time goal. Apparently, during this initial stage, our aim is to raise many open questions than to actually answer ones.

For the following stages, we will prove the concepts using real data in the power grids. The high-dimensional statistic MSR, illustrated as the contour line mentioned in Case 4, will be programmed as a friendly real-time 3D animation to visualize the status and trend of the whole system in . One wonders if this new direction will be far-reaching in years to come toward the age of Big Data.

## Appendix A
## The Grid Network Structures G1, G2 and G3

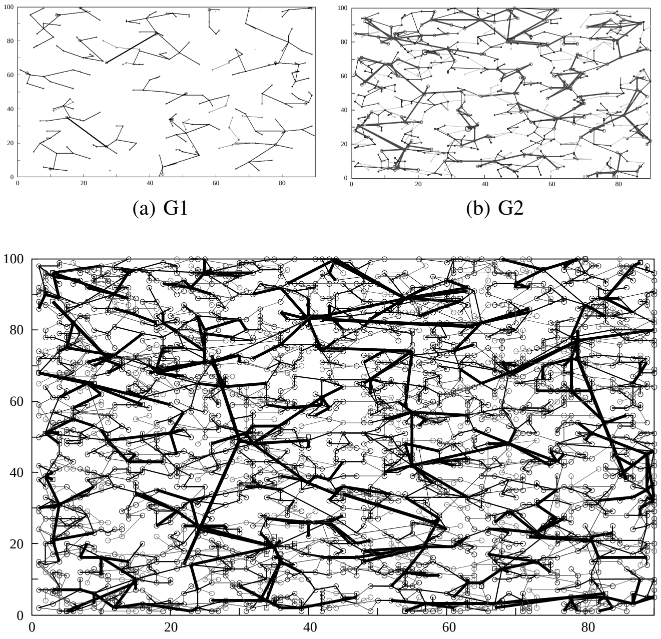
(a) G1 (b) G2

(c) G3

Fig. 11: Simulation of network structures for three generations of power systems. The above twos are G1—Small-scale isolated grids, and G2—Large-scale interconnected power grids, respectively; and the below one is G3—Smart grids, which have complex network structures without clear-cut partitioning.

## Appendix B
## Event Series for Five Case Studies

TABLE II: Series of Events for Case 1

| | | | |
|---|---|---|---|
| $t$ | [001 : 550] | [551 : 1100] | [1101 : 1650] |
| $P_{\text{Bus-59}}$ | 0 | 200 | 0 |
| $t$ | [1651 : 2200] | [2201 : 2500] | |
| $P_{\text{Bus-59}}$ | 1500 | 0 | |

*$t$: (s), $P_{\text{Bus-59}}$: (MW)

TABLE III: Series of Events for Case 2

| | | | |
|---|---|---|---|
| $t$ | [001 : 300] | [301 : 600] | [601 : 900] |
| $P_{\text{Bus-59}}$ | 0 | 200 | 250 |
| $t$ | [901 : 1200] | [1201 : 1500] | [1501 : 1800] |
| $P_{\text{Bus-59}}$ | 800 | 850 | 2000 |
| $t$ | [1801 : 2100] | [2101 : 2400] | [2401 : 2500] |
| $P_{\text{Bus-59}}$ | 2540 | 2555 | 3500 |

*$t$: (s), $P_{\text{Bus-59}}$: (MW)

TABLE IV: Series of Events for Case 4

| | | | |
|---|---|---|---|
| $t$ | [001 : 300] | [301 : 700] | [701 : 1000] |
| $P_{\text{Bus-117}}$ | 0 | 150 | $t/2 - 200$ |

*$t$: (s), $P_{\text{Bus-117}}$: (MW)

TABLE V: Series of Events for Case 5

| | | | |
|---|---|---|---|
| $t$ | [1000 : 1500] | [3000 : 3500] | [5000 : 5500] |
| Event | A $\to$ G | AB $\to$ G | B $\to$ G |
| $t$ | [7000 : 7500] | [9000 : 11000] | [13000 : 13500] |
| Event | C $\to$ G | BCS OPEN | ABC $\to$ G |

*$t$: (ms)

# APPENDIX C

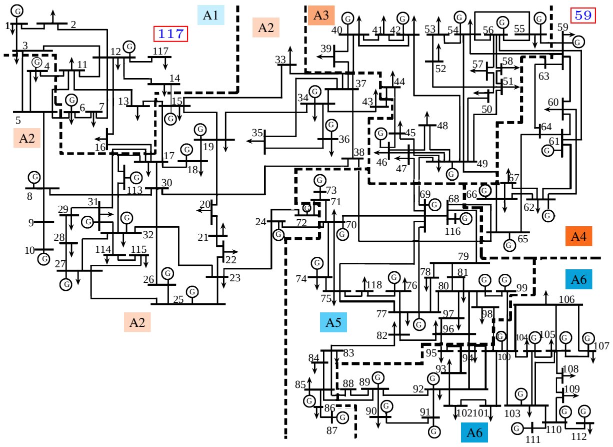


Fig. 12: Partitioning network for IEEE 118-bus system. There are six partitions, i.e. A1, A2, A3, A4, A5, and A6. Under group-work mode, each region has its own regional control center served as the assistant to the global control center.

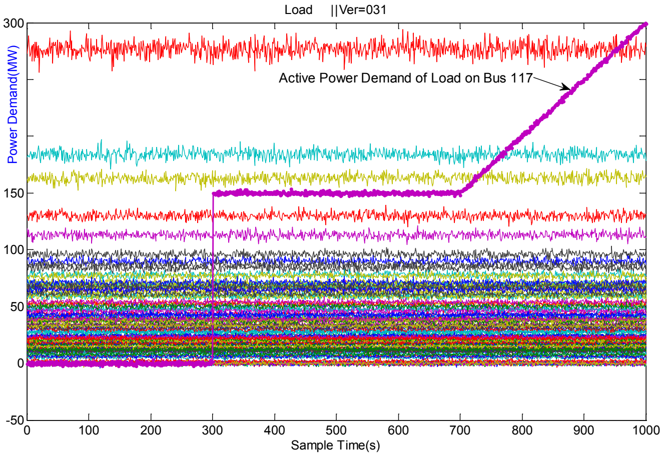


Fig. 13: Load change of grid ($\gamma_{\text{Acc}} = 1$, $\gamma_{\text{Mul}} = 0.02$) for Case 4

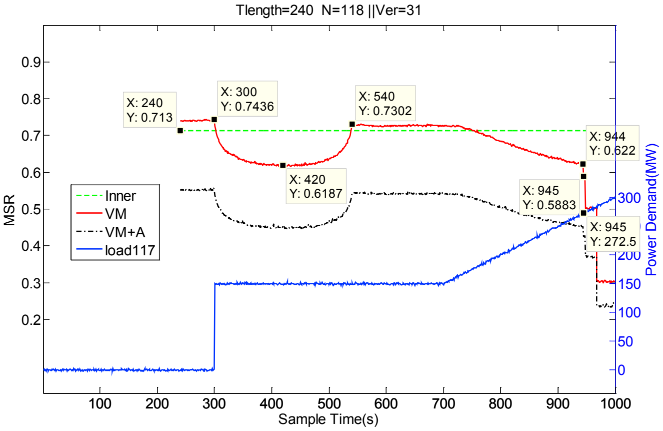


Fig. 14: the Global MSR ($P_{\text{max\_Bus-117}} = 272.5$ MW)

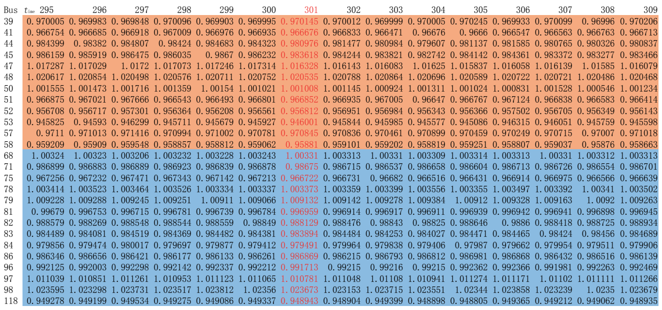

| Bus $t_{\text{ime}}$ | 295 | 296 | 297 | 298 | 299 | 300 | 301 | 302 | 303 | 304 | 305 | 306 | 307 | 308 | 309 |
|---|---|---|---|---|---|---|---|---|---|---|---|---|---|---|---|
| 39 | 0.970005 | 0.969983 | 0.969848 | 0.970096 | 0.969903 | 0.969995 | 0.970145 | 0.970012 | 0.969999 | 0.970005 | 0.970245 | 0.969933 | 0.970099 | 0.96996 | 0.970206 |
| 41 | 0.966754 | 0.966685 | 0.966918 | 0.967009 | 0.966976 | 0.966935 | 0.966676 | 0.966833 | 0.966471 | 0.96676 | 0.9666 | 0.966547 | 0.966563 | 0.966763 | 0.966713 |
| 44 | 0.984399 | 0.98382 | 0.984807 | 0.98424 | 0.984683 | 0.984323 | 0.980976 | 0.981477 | 0.980984 | 0.979607 | 0.981137 | 0.981585 | 0.980765 | 0.980326 | 0.980837 |
| 45 | 0.986159 | 0.985919 | 0.986475 | 0.986035 | 0.9867 | 0.986232 | 0.983618 | 0.984244 | 0.983821 | 0.982742 | 0.984142 | 0.984361 | 0.983372 | 0.983277 | 0.983466 |
| 47 | 1.017287 | 1.017029 | 1.0172 | 1.017073 | 1.017246 | 1.017314 | 1.016328 | 1.016143 | 1.016083 | 1.01625 | 1.015837 | 1.016058 | 1.016139 | 1.01585 | 1.016079 |
| 48 | 1.020617 | 1.020854 | 1.020498 | 1.020576 | 1.020711 | 1.020752 | 1.020535 | 1.020788 | 1.020864 | 1.020696 | 1.020589 | 1.020722 | 1.020721 | 1.020486 | 1.020468 |
| 50 | 1.001555 | 1.001473 | 1.001716 | 1.001359 | 1.00154 | 1.001021 | 1.001008 | 1.001145 | 1.000924 | 1.001311 | 1.001024 | 1.000831 | 1.001528 | 1.000546 | 1.001234 |
| 51 | 0.966875 | 0.967021 | 0.967666 | 0.966543 | 0.966493 | 0.966801 | 0.966852 | 0.966935 | 0.967005 | 0.96647 | 0.966767 | 0.967124 | 0.966838 | 0.966583 | 0.966414 |
| 52 | 0.956708 | 0.956717 | 0.957301 | 0.956364 | 0.956208 | 0.956561 | 0.956812 | 0.956951 | 0.956984 | 0.956343 | 0.956366 | 0.957502 | 0.956705 | 0.956349 | 0.956143 |
| 53 | 0.945825 | 0.94593 | 0.946299 | 0.945711 | 0.945679 | 0.945927 | 0.946001 | 0.945844 | 0.945985 | 0.945577 | 0.945086 | 0.946315 | 0.946051 | 0.945759 | 0.945598 |
| 57 | 0.9711 | 0.971013 | 0.971416 | 0.970994 | 0.971002 | 0.970781 | 0.970845 | 0.970836 | 0.970461 | 0.970899 | 0.970459 | 0.970249 | 0.970715 | 0.97007 | 0.971018 |
| 58 | 0.959209 | 0.95909 | 0.959548 | 0.958857 | 0.958812 | 0.959062 | 0.95881 | 0.959101 | 0.959202 | 0.958819 | 0.959251 | 0.958807 | 0.959037 | 0.95876 | 0.958663 |
| 68 | 1.00324 | 1.00323 | 1.003206 | 1.003232 | 1.003228 | 1.003243 | 1.00331 | 1.003313 | 1.00331 | 1.003309 | 1.003314 | 1.003313 | 1.00331 | 1.003312 | 1.003313 |
| 71 | 0.986899 | 0.986883 | 0.986889 | 0.986923 | 0.986839 | 0.986878 | 0.98675 | 0.986715 | 0.986537 | 0.986658 | 0.986604 | 0.986713 | 0.986726 | 0.986554 | 0.986701 |
| 75 | 0.967256 | 0.967232 | 0.967471 | 0.967343 | 0.967142 | 0.967213 | 0.966722 | 0.966731 | 0.96682 | 0.966516 | 0.966431 | 0.966914 | 0.966975 | 0.966566 | 0.966639 |
| 78 | 1.003414 | 1.003523 | 1.003464 | 1.003526 | 1.003334 | 1.003337 | 1.003373 | 1.003359 | 1.003399 | 1.003556 | 1.003355 | 1.003497 | 1.003392 | 1.00341 | 1.003502 |
| 79 | 1.009228 | 1.009288 | 1.009245 | 1.009251 | 1.00911 | 1.009066 | 1.009132 | 1.009142 | 1.009278 | 1.009384 | 1.00912 | 1.009328 | 1.009163 | 1.0092 | 1.009263 |
| 81 | 0.99679 | 0.996753 | 0.996715 | 0.996781 | 0.996739 | 0.996784 | 0.996959 | 0.996914 | 0.996917 | 0.996911 | 0.996939 | 0.996942 | 0.996941 | 0.996898 | 0.996945 |
| 82 | 0.988579 | 0.988269 | 0.988548 | 0.988544 | 0.988559 | 0.98849 | 0.988129 | 0.988476 | 0.98843 | 0.98825 | 0.988646 | 0.9886 | 0.988418 | 0.988725 | 0.988934 |
| 83 | 0.984489 | 0.984081 | 0.984519 | 0.984369 | 0.984482 | 0.984381 | 0.983894 | 0.984484 | 0.984253 | 0.984027 | 0.984471 | 0.984465 | 0.98424 | 0.98456 | 0.984689 |
| 84 | 0.979856 | 0.979474 | 0.980017 | 0.979697 | 0.979877 | 0.979412 | 0.979491 | 0.979964 | 0.979838 | 0.979406 | 0.97987 | 0.979662 | 0.979954 | 0.979511 | 0.979906 |
| 86 | 0.986346 | 0.986656 | 0.986421 | 0.986177 | 0.986133 | 0.986261 | 0.986869 | 0.986215 | 0.986793 | 0.986812 | 0.986981 | 0.986868 | 0.986432 | 0.986516 | 0.986139 |
| 96 | 0.992125 | 0.992003 | 0.992298 | 0.992142 | 0.992337 | 0.992212 | 0.991713 | 0.99215 | 0.99216 | 0.99215 | 0.992362 | 0.992366 | 0.991981 | 0.992263 | 0.992469 |
| 97 | 1.011039 | 1.010851 | 1.011261 | 1.010953 | 1.011123 | 1.011065 | 1.010781 | 1.011048 | 1.01108 | 1.010941 | 1.011274 | 1.011171 | 1.01102 | 1.011111 | 1.011266 |
| 98 | 1.023595 | 1.023298 | 1.023731 | 1.023517 | 1.023812 | 1.02356 | 1.023673 | 1.023153 | 1.023715 | 1.023551 | 1.02344 | 1.023858 | 1.023239 | 1.0235 | 1.023679 |
| 118 | 0.949278 | 0.949199 | 0.949534 | 0.949275 | 0.949086 | 0.949337 | 0.948943 | 0.948904 | 0.949399 | 0.948898 | 0.948805 | 0.949365 | 0.949212 | 0.949062 | 0.948935 |

(a) Raw Data $\hat{\mathbf{V}}$

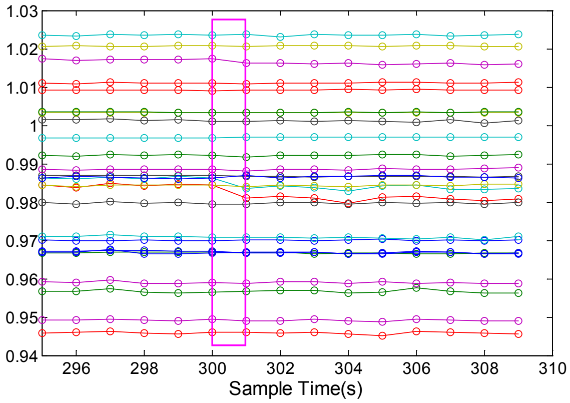


(b) Low-dimensional Visualization of $\hat{\mathbf{V}}$

Fig. 15: Raw Data $\hat{\mathbf{V}}$ and their Visualization around Sampling time $t_s = 300$ s(Orange for A3, and Blue for A5)

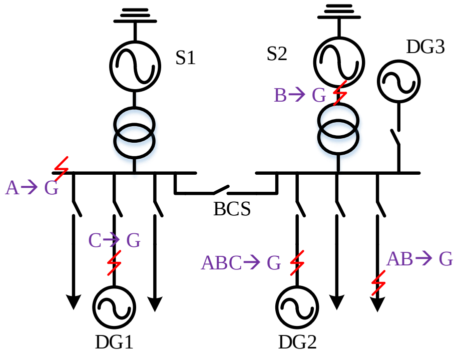


Fig. 16: Fault Model for Case 5

# REFERENCES

[1] Nature, "Big data (specials)," Sep 2008, http://www.nature.com/news/specials/bigdata/index.html.

[2] Science, "Special online collection: Dealing with data," Feb 2011, http://www.sciencemag.org/site/special/data/.

[3] T. A. Brody, J. Flores, J. B. French, P. Mello, A. Pandey, and S. S. Wong, "Random-matrix physics: spectrum and strength fluctuations," *Reviews of Modern Physics*, vol. 53, no. 3, p. 385, 1981.

[4] L. Laloux, P. Cizeau, M. Potters, and J.-P. Bouchaud, "Random matrix theory and financial correlations," *International Journal of Theoretical and Applied Finance*, vol. 3, no. 03, pp. 391–397, 2000.

[5] H. Chen, R. H. Chiang, and V. C. Storey, "Business intelligence and analytics: From big data to big impact." *MIS quarterly*, vol. 36, no. 4, pp. 1165–1188, 2012.

[6] D. Howe, M. Costanzo, P. Fey, T. Gojobori, L. Hannick, W. Hide, D. P. Hill, R. Kania, M. Schaeffer, S. St Pierre *et al.*, "Big data: The future of biocuration," *Nature*, vol. 455, no. 7209, pp. 47–50, 2008.

[7] R. Qiu and M. Wicks, *Cognitive Networked Sensing and Big Data*. Springer, 2013.

[8] C. Zhang and R. C. Qiu, "Data modeling with large random matrices in a cognitive radio network testbed: Initial experimental demonstrations with 70 nodes," *arXiv preprint arXiv:1404.3788*, 2014.

[9] X. Li, F. Lin, and R. C. Qiu, "Modeling massive amount of experimental data with large random matrices in a real-time UWB-MIMO system," *CoRR*, vol. abs/1404.4078, 2014. [Online]. Available: http://arxiv.org/abs/1404.4078

[10] IBM, "The four vs of big data." [EB/OL], http://www.ibmbigdatahub.com/infographic/four-vs-big-data.

[11] R. Qiu and P. Antonik, *Smart Grid and Big Data*. John Wiley and Sons, 2014.

[12] IBM, "Managing big data for smart grids and smart meters," May 2009.

[13] M. Kezunovic, L. Xie, and S. Grijalva, "The role of big data in improving power system opera-tion and protection," in *Bulk Power System Dynamics and Control-IX Optimization, Security and Control of the Emerging Power Grid (IREP), 2013 IREP Symposium*. IEEE, 2013, pp. 1–9.

[14] N. Kanao, M. Yamashita, H. Yanagida, M. Mizukami, Y. Hayashi, and J. Matsuki, "Power system harmonic analysis using state-estimation method for japanese field data," *Power Delivery, IEEE Transactions on*, vol. 20, no. 2, pp. 970–977, 2005.

[15] D. Alahakoon and X. Yu, "Advanced analytics for harnessing the power of smart meter big data," in *Intelligent Energy Systems (IWIES), 2013 IEEE International Workshop on*. IEEE, 2013, pp. 40–45.

[16] W. XU and J. YONG, "Power disturbance data analytics–new application of power quality monitoring data," *Proceedings of the CSEE*, vol. 19, p. 013, 2013.

[17] R. C. Qiu, Z. Hu, H. Li, and M. C. Wicks, *Cognitive radio communication and networking: Principles and practice*. John Wiley & Sons, 2012.

[18] V. A. Marčenko and L. A. Pastur, "Distribution of eigenvalues for some sets of random matrices," *Sbornik: Mathematics*, vol. 1, no. 4, pp. 457–483, 1967.

[19] G. Pan, Q.-M. Shao, and W. Zhou, "Universality of sample covariance matrices: Clt of the smoothed empirical spectral distribution," *arXiv preprint arXiv:1111.5420*, 2011.

[20] A. Guionnet, M. Krishnapur, and O. Zeitouni, "The single ring theorem," *arXiv preprint arXiv:0909.2214*, 2009.

[21] F. Benaych-Georges and J. Rochet, "Outliers in the single ring theorem," *arXiv preprint arXiv:1308.3064*, 2013.

[22] J. R. Ipsen and M. Kieburg, "Weak commutation relations and eigenvalue statistics for products of rectangular random matrices," *Physical Review E*, vol. 89, no. 3, p. 032106, 2014.

[23] X. Zhou, S. Chen, and Z. Lu, "Review and prospect for power system development and related technologies: a concept of three-generation power systems," *Proceedings of the CSEE*, vol. 22, pp. 1–11, 2013.

[24] S. MEI, y. GONG, and f. LIU, "The evolution model of three generation power systems and characteristic analysis," *Proceedings of the CSEE*, vol. 7, pp. 1003–1012, 2014.

[25] X. He, Q. Ai, Z. Yu, Y. Xu, and J. Zhang, "Power system evolution and aggregation theory under the view of power ecosystem," *Power System Protection and Control*, vol. 22, pp. 100–107, 2014.

[26] R. C. Qiu, Z. Hu, Z. Chen, N. Guo, R. Ranganathan, S. Hou, and G. Zheng, "Cognitive radio network for the smart grid: experimental system architecture, control algorithms, security, and microgrid testbed," *Smart Grid, IEEE Transactions on*, vol. 2, no. 4, pp. 724–740, 2011.

[27] H. Li, S. Gong, L. Lai, Z. Han, R. C. Qiu, and D. Yang, "Efficient and secure wireless communications for advanced metering infrastructure in smart grids," *Smart Grid, IEEE Transactions on*, vol. 3, no. 3, pp. 1540–1551, 2012.

[28] H. Li, L. Lai, and R. C. Qiu, "Scheduling of wireless metering for power market pricing in smart grid," *Smart Grid, IEEE Transactions on*, vol. 3, no. 4, pp. 1611–1620, 2012.

[29] D. Baigent, M. Adamiak, R. Mackiewicz, and G. M. G. M. SISCO, "Iec 61850 communication networks and systems in substations: an overview for users," in *Proceedings of the VIII simposio iberoamericano sobre proteccion de sistemas electricos de potencia, Monterey, Mexico, Citeseer*, 2004.

[30] R.-F. Yuan, Q. Ai, and X. He, "Research on dynamic load modelling based on power quality monitoring system," *Generation, Transmission & Distribution, IET*, vol. 7, no. 1, pp. 46–51, 2013.

[31] Q. Ai, X. Wang, and X. He, "The impact of large-scale distributed generation on power grid and microgrids," *Renewable Energy*, vol. 62, pp. 417–423, 2014.

[32] Y. Ji, "Multi-agent system based control of virtual power plant and its application in smart grid," Master's thesis, Shanghai Jiaotong University, 2011.

[33] X. He, Q. Ai, P. Yuan, and X. Wang, "The research on coordinated operation and cluster management for multi-microgrids," in *Sustainable Power Generation and Supply (SUPERGEN 2012), International Conference on*. IET, 2012, pp. 1–3.

[34] X. Ni, Q. Ruan, and S. Mei, "A new network partitioning algorithm based on complex network theory and its application in shanghai power grid," *POWER SYSTEM TECHNOLOGY-BEIJING-*, vol. 31, no. 9, p. 6, 2007.

[35] R. Zimmerman, C. Murillo-Sánchez, and D. Gan, "Matpower users manual, version 4.1," *Power Systems Engineering Research Center*, 2011.

[36] Y. Zhao, Y. An, and Q. Ai, "Research on size and location of distributed generation with vulnerable node

identification in the active distribution network," 2014.
[37] W. Huang, T. Nengling, X. Zheng, C. Fan, X. Yang, and B. J. Kirby, "An impedance protection scheme for feeders of active distribution networks," 2014.
